# Supplementary material for: UniAudio: An Audio Foundation Model Toward Universal Audio Generation
Source: arXiv:2310.00704 source file (2024-12-10)
Supplement: Supplementary file 1 [file 6_appendix_related_work.tex]

\section{Related works} \label{appendix:related_work}
\subsection{Self-Supervised Learning in Audio}
Learning the useful representation by self-supervised learning (SSL) \cite{baevski2020wav2vec,baevski2022data2vec}
has been demonstrated as a effective way to using large-scale audio data. HuBERT \cite{hsu2021hubert} aims to capture rich contextual information from raw audio signals, which is trained use a masked prediction objective. Furthermore, it incorporates an offline clustering process (such as K-means) to obtain aligned target labels for
a prediction loss similar to BERT. Recently, neural audio codec models \cite{zeghidour2021soundstream,defossez2022high,yang2023hifi}got a lot of attention in audio generation tasks. Audio Codec models can be trained on audio-only dataset, and it compresses continuous audio data into discrete representation, which is suitable to be modeled by language models. In this study, we explore to train a universal audio codec models that can compress different types of audio (such as speech, sound, music and sing data) into one shared discrete latent space, so that we can use a universal audio language models to generate them. 
\subsection{Audio Language Models}
Neural language models have demonstrated remarkable abilities for different tasks \cite{OpenAI}, such as dialog with humans and solving math problems. In audio fields, Jukebox adopts a hierarchical approach to generate tokens, then recover the music based on tokens. 'textless NLP' series works that model language directly in the speech domain, by using discrete speech representation for self-supervised learning. But their audio quality remains limited. AudioLM is the first model to generate long-term coherence and high-quality audio, which makes use of Soundstream to compress audio into latent space and two cascaded decoder-only models to generate tokens. Inspired by AudioLM, a lot of works attempt to use audio language model to generate speech \cite{wang2023neural,kharitonov2023speak,huang2023make}, music \cite{agostinelli2023musiclm,copet2023simple}, sound \cite{kreuk2022audiogen}, sing voice \cite{huang2023make}. However, currently works both focus on using large-scale data to train a audio language model for sing task, which is far from the neural language model's target. In this study, we make the following assumption: (1) a universal audio language model can solve all of audio-related generation tasks. (2) multi-tasks training can bring benifits than single task training when we found a proper latent space that can be shared by different type audio data.
\subsection{Zero-shot Audio Related Tasks}
\textbf{Zero-shot Speech/Sing Synthesis}
Previous TTS models (such as Tactron \cite{wang2017tacotron} and FastSpeech \cite{ren2019fastspeech}) typically convert input text into mel-spectrogram, then a vocoder is used to recover the waveform from mel-spectrogram. Recently, zero-shot TTS got a lot of attention due to it can imitate any one's voice. YourTTS \cite{casanova2022yourtts} is the one of representive works, which is built upon VITS with several novel modifications. However, the voice clone ability is still poor due to the training data is not enough. VALL-E \cite{wang2023neural} is the first work to consider using large-scale data to help realize zero-shot TTS. Following VALL-E, SPEARTTS \cite{kharitonov2023speak}, NauturalSpeech2, Make-A-Voice, Mega-TTS and VoiceBox also consider using large-scale data to realize zero-shot TTS. Most of the Sing voice synthesis (SVS) systems \cite{liu2022diffsinger} focus on using a network transfer the music score into mel-spectrogram, then training a vocoder that translate mel-spectrogram into waveform. Make-A-Voice \cite{huang2023make} proposes to a two stage method to generate sing voice in discrete latent space. However, Make-A-Voice still need to train a special vocoder to decode sing. In this study, we explore using a model directly generating sing conditioned on text, MIDI and prompt.

\textbf{Zero-shot Voice/Sing Conversion}
Zero-shot any-to-any voice or sing conversion \cite{casanova2022yourtts,lei2022glow,lin2021s2vc} have been widely discuss in literature. Previous works focus on decoupling the timbre information from audio, so that the speaker's timbre can be conversion easily by change the timbre representations. Recently, many works \cite{wang2023lm,huang2023make} ignore the decoupling process, instead they introduce more speaker data and using a language model to reconstruct the target audio based on content information and a 3 seconds prompt audio. 

\textbf{Zero-shot Speech Enhancement/Extraction}
In speech front-end fields, generative models are not the mainstream methods. For example, speech enhancement and separation tasks are mainly solved by discriminate models. Although some researches have explored using generative methods, such as GAN \cite{phan2020improving} or Diffusion models \cite{lu2022conditional,richter2023speech} to solve these tasks. The performance still cannot compare with the SOTA discriminate models. In this study, we try to solve the speech separation tasks by large-scale audio language models training. We demonstrate that our model can significantly improve the generalization.

\textbf{Zero-shot Text to Sound/Music}
Text to audio generation is a rising task that has seen great advances recently. DiffSound \cite{yang2023diffsound}
is the first work to explore generate sound effect based text description. AudioGen \cite{kreuk2022audiogen} propose to generate sound by training a audio language model. Another line in text-to-sound is adopt latent diffusion models, such as Make-An-Audio \cite{huang2023make}, AudioLMD \cite{liu2023audioldm}, Tango\cite{ghosal2023text}, Make-an-Audio 2 \cite{huang2023make}, AUDIT \cite{wang2023audit}. Text-to-music generation also attracts great attention, such as MusicLM \cite{agostinelli2023musiclm}, Riffusion \cite{Forsgren_Martiros_2022}, Mousai \cite{schneider2023mo}, Noise2Music \cite{huang2023noise2music}, Melody \cite{lam2023efficient} and MusicGen \cite{copet2023simple}. AudioGen and MusicGen are the most similar to ours. Although the open source code is available, we find that training such models need large GPU resources due to they formulation results in long sequence problem. In this study, we also propose to use audio language model to generate sound or music, the difference is that our model can effectively reduce the sequence length. In fact, our model can be trained by one 16G GPU.
